# Supplementary material for: Image Restoration by Deep Projected GSURE
Source: arXiv:2102.02485 source file (2021-02-04)
Supplement: Supplementary file 1 [file 06_supp.tex]

In the following, we:

\begin{itemize}
    \item Present the DIP-P\&P and GSURE-P\&P results on Set14.
    \item Show additional visual comparison of the different methods.
\end{itemize}

\section{P\&P On Set14}
In this section, we present the results of the P\&P approach (that uses BM3D prior imposed by BM3D denoiser) tested on Set14 with all the scenarios we presented in the article, as can be seen in Tables \ref{table:PnP_deblur_Set14} and \ref{table:PnP_SR_Set14}.

\begin{table}[ht]
\small
\caption{Deblurring results on Set14 (averaged PSNR) of the P\&P based methods for the different scenarios} \label{table:PnP_deblur_Set14}   
\centering
    \begin{tabular}{ | c | c | c | c | c | c |}
    \hline
    Scenario& P\&P          & P\&P-DIP  & P\&P-GSURE \\ \hline
        1   &  30.72        &   27.49   & \textbf{30.97}\\ \hline
        2   &  28.27        &   27.46   & \textbf{28.92}\\ \hline
        3   &  \textbf{30.31} &   25.85   & 27.58\\ \hline
        4   &  29.29        &   28.85   & \textbf{29.7}\\ \hline
        5   &  28.66 &   27.55   & \textbf{28.71} \\ \hline
        6   &  33.69        &   29.74   & \textbf{34.45}\\ \hline
    \end{tabular}
\end{table}

\begin{table}[ht]
\small
\caption{SR results on Set14 (averaged PSNR) of the P\&P based methods for the different scenarios} \label{table:PnP_SR_Set14}   
\centering
    \begin{tabular}{ | c | c | c | c | c | c |}
    \hline
    Scenario& P\&P   & P\&P-DIP & P\&P-GSURE \\ \hline
        1   &  26.12 &  26.67   & \textbf{29.77}\\ \hline
        2   &  25.20 &  25.59   & \textbf{25.93}\\ \hline
        3   &  29.57 &  29.14   & \textbf{29.58}\\ \hline
        4   &  26.90 &  27.19   & \textbf{27.00}\\ \hline
        5   &  27.90 &  28.47   & \textbf{28.77}\\ \hline
        6   &  25.63 &  26.30   & \textbf{26.46}\\ \hline
    \end{tabular}
\end{table}

As it can be seen from the tables above, replacing the least-squares term in DIP with the P-GSURE term improves the reconstruction results dramatically as well as achieving better results than the standard P\&P denoisers approach in most cases, in both SR and deblurring cases.

\section{Visual Comparison}
In this section we compare the different methods perceptually.

\begin{figure}[ht]
    \centering
    \begin{subfigure}{0.45\linewidth}
        \centering
        \includegraphics[trim={0pt, 0pt, 0pt, 50pt} ,clip,width=150pt]{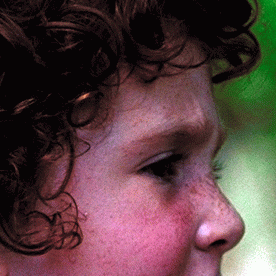}
        \caption{Original image (cropped)}
    \end{subfigure}
    \begin{subfigure}{0.45\linewidth}
        \centering
        \includegraphics[trim={0pt, 0pt, 0pt, 50pt}, clip,width=150pt]{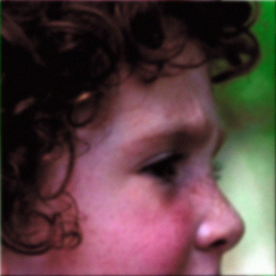}
        \caption{Blurred}
    \end{subfigure}\\
    \begin{subfigure}{0.45\linewidth}
        \centering
        \includegraphics[trim={0pt, 0pt, 0pt, 50pt} ,clip,width=150pt]{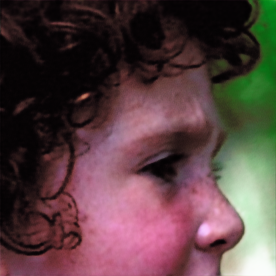}
        \caption{DIP}   
    \end{subfigure}
    \begin{subfigure}{0.45\linewidth}
        \centering
        \includegraphics[trim={0pt, 0pt, 0pt, 50pt} ,clip,width=150pt]{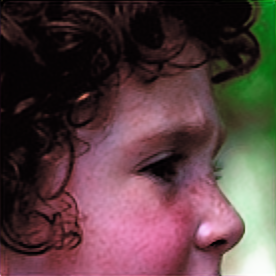}
        \caption{P-GSURE}       
    \end{subfigure}\\
    \begin{subfigure}{0.33\linewidth}
        \centering
        \includegraphics[trim={0pt, 0pt, 0pt, 50pt} ,clip,width=150pt]{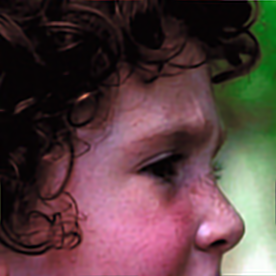}
        \caption{P\&P ADMM}   
    \end{subfigure}
    \begin{subfigure}{0.33\linewidth}
        \centering
        \includegraphics[trim={0pt, 0pt, 0pt, 50pt} ,clip,width=150pt]{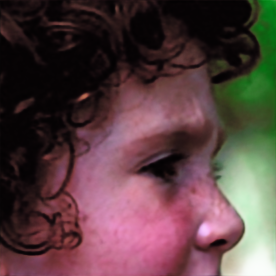}
        \caption{DIP-P\&P}
    \end{subfigure}
    \begin{subfigure}{0.33\linewidth}
        \centering
        \includegraphics[trim={0pt, 0pt, 0pt, 50pt} ,clip,width=150pt]{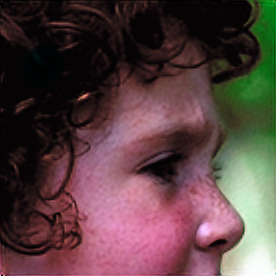}
        \caption{P-GSURE P\&P}  
    \end{subfigure}
    \caption{Deblurring of the face image from Set14, blurred using the model of scenario 5. (a) The original image cropped (b) The observed blurry and noisy image (c) Reconstruction using DIP (d) Reconstruction using P-GSURE (proposed method) (e) Reconstruction using P\&P-ADMM method (using BM3D prior) (f) Reconstruction using DIP based P\&P-ADMM (g) Reconstruction using P-GSURE based P\&P-ADMM (proposed method).}
    \label{fig:comparison_deblur_scenario5}
\end{figure}

\begin{figure}[ht]
    \centering
    \begin{subfigure}{0.45\linewidth}
        \centering
        \includegraphics[trim={200pt, 90pt, 60pt, 100pt} ,clip,width=150pt]{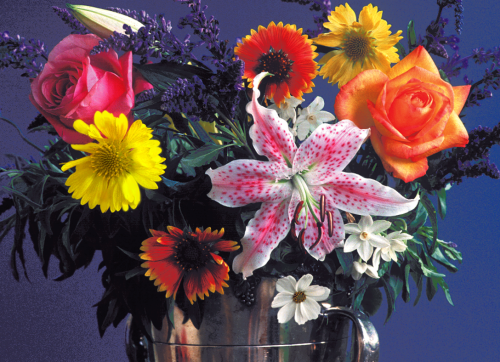}
        \caption{Original image (cropped)}    
    \end{subfigure}
    \begin{subfigure}{0.45\linewidth}
        \centering
        \includegraphics[trim={200pt, 90pt, 60pt, 100pt}, clip,width=150pt]{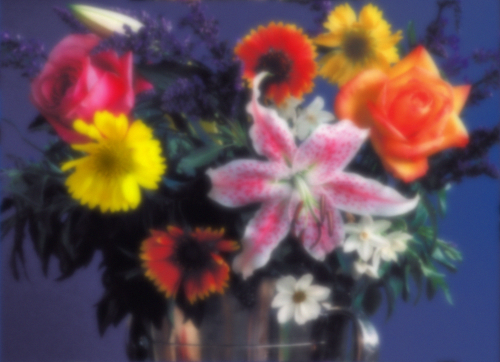}
        \caption{Blurred}
    \end{subfigure}\\
    \begin{subfigure}{0.45\linewidth}
        \centering
        \includegraphics[trim={200pt, 90pt, 60pt, 100pt} ,clip,width=150pt]{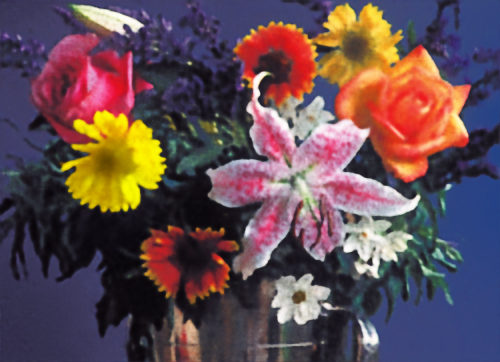}
        \caption{DIP}
    \end{subfigure}
    \begin{subfigure}{0.45\linewidth}
        \centering
        \includegraphics[trim={200pt, 90pt, 60pt, 100pt} ,clip,width=150pt]{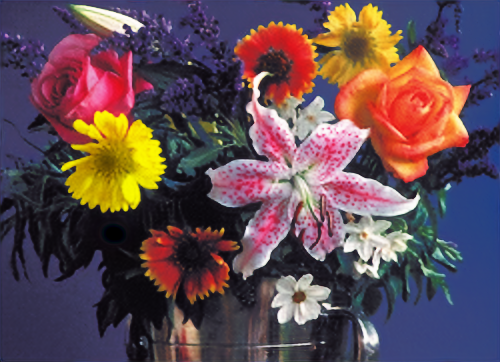}
        \caption{P-GSURE}
    \end{subfigure}\\
    \begin{subfigure}{0.33\linewidth}
        \centering
        \includegraphics[trim={200pt, 90pt, 60pt, 100pt} ,clip,width=150pt]{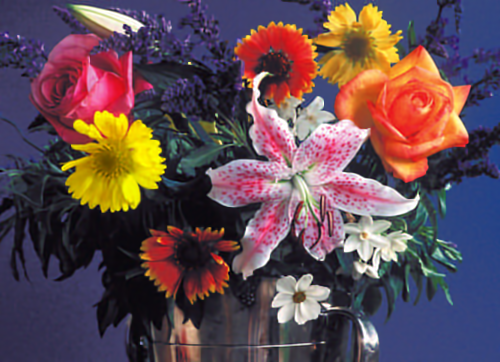}
        \caption{P\&P ADMM}
    \end{subfigure}
    \begin{subfigure}{0.33\linewidth}
        \centering
        \includegraphics[trim={200pt, 90pt, 60pt, 100pt} ,clip,width=150pt]{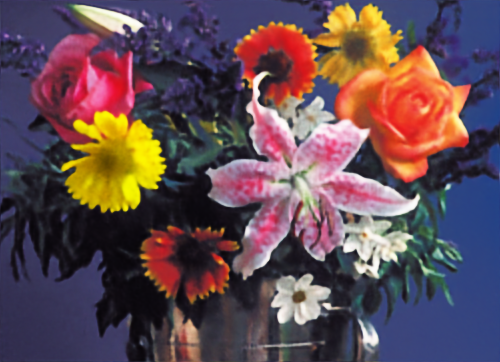}
        \caption{DIP-P\&P} 
    \end{subfigure}
    \begin{subfigure}{0.33\linewidth}
        \centering
        \includegraphics[trim={200pt, 90pt, 60pt, 100pt} ,clip,width=150pt]{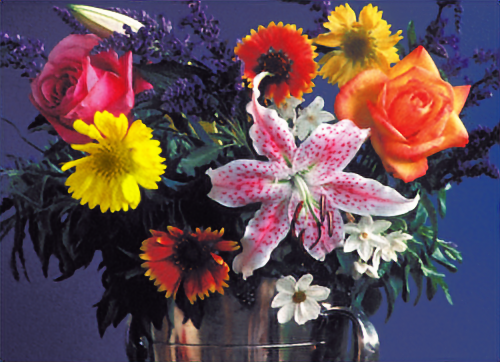}
        \caption{P-GSURE P\&P}
    \end{subfigure}
    \caption{Deblurring of the flowers image from Set14, blurred using the model of scenario 1. (a) The original image cropped (b) The observed blurry and noisy image (c) Reconstruction using DIP (d) Reconstruction using P-GSURE (proposed method) (e) Reconstruction using P\&P-ADMM method (using BM3D prior) (f) Reconstruction using DIP based P\&P-ADMM (g) Reconstruction using P-GSURE based P\&P-ADMM (proposed method).}
    \label{fig:comparison_deblur_scenario1}
\end{figure}

\begin{figure}[ht]
    \centering
    \begin{subfigure}{0.45\linewidth}
        \centering
        \includegraphics[trim={200pt, 50pt, 0pt, 60pt} ,clip,width=150pt]{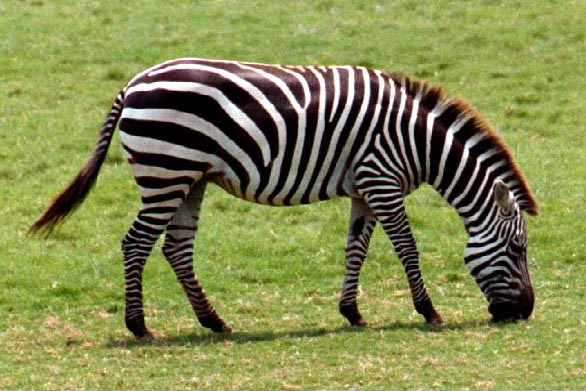}
        \caption{Original image (cropped)}
    \end{subfigure}
    \begin{subfigure}{0.45\linewidth}
        \centering
        \includegraphics[trim={200pt, 50pt, 0pt, 60pt}, clip,width=150pt]{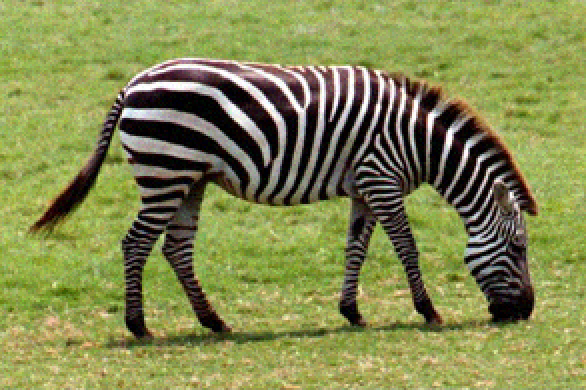}
        \caption{Blurred}
    \end{subfigure}\\
    \begin{subfigure}{0.45\linewidth}
        \centering
        \includegraphics[trim={200pt, 50pt, 0pt, 60pt} ,clip,width=150pt]{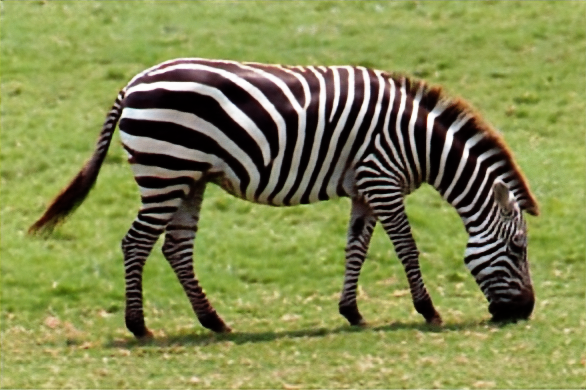}
        \caption{DIP}
    \end{subfigure}
    \begin{subfigure}{0.45\linewidth}
        \centering
        \includegraphics[trim={200pt, 50pt, 0pt, 60pt} ,clip,width=150pt]{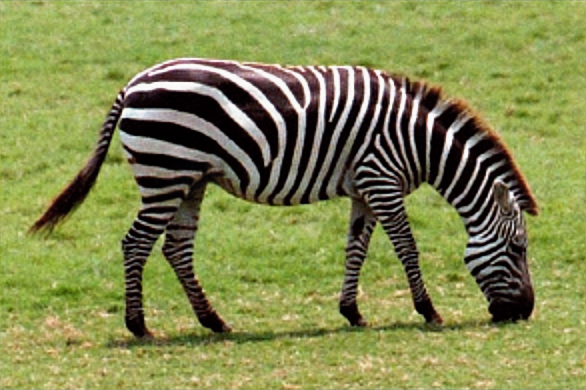}
        \caption{P-GSURE}
    \end{subfigure}\\
    \begin{subfigure}{0.33\linewidth}
        \centering
        \includegraphics[trim={200pt, 50pt, 0pt, 60pt} ,clip,width=150pt]{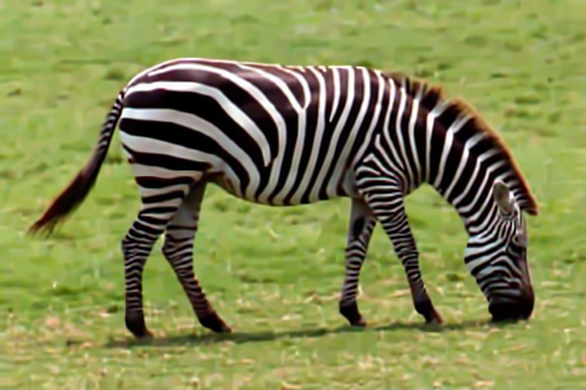}
        \caption{P\&P ADMM}
    \end{subfigure}
    \begin{subfigure}{0.33\linewidth}
        \centering
        \includegraphics[trim={200pt, 50pt, 0pt, 60pt} ,clip,width=150pt]{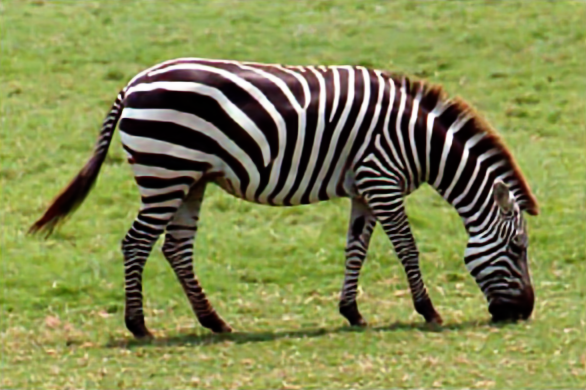}
        \caption{DIP-P\&P}
    \end{subfigure}
    \begin{subfigure}{0.33\linewidth}
        \centering
        \includegraphics[trim={200pt, 50pt, 0pt, 60pt} ,clip,width=150pt]{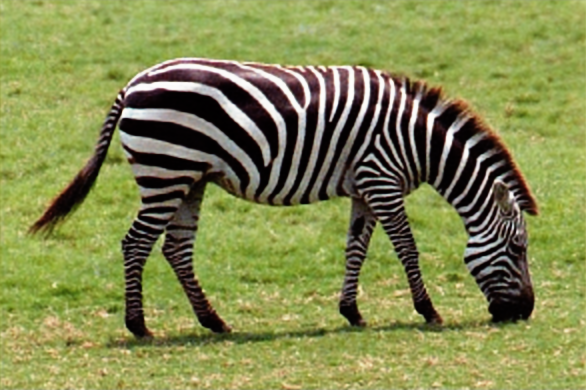}
        \caption{P-GSURE P\&P}
    \end{subfigure}
    \caption{SR of the zebra image from Set14, down-sampled using the model from scenario 5. (a) The original image cropped (b) The observed LR noisy image (c) Reconstruction using DIP (d) Reconstruction using P-GSURE (proposed method) (e) Reconstruction using P\&P-ADMM method (using BM3D prior) (f) Reconstruction using DIP based P\&P-ADMM (g) Reconstruction using P-GSURE based P\&P-ADMM (proposed method).}
    \label{fig:comparison_SR_scenario5}
\end{figure}

\begin{figure}[ht]
    \centering
    \begin{subfigure}{0.45\linewidth}
        \centering
        \includegraphics[trim={200pt, 50pt, 0pt, 150pt} ,clip,width=150pt]{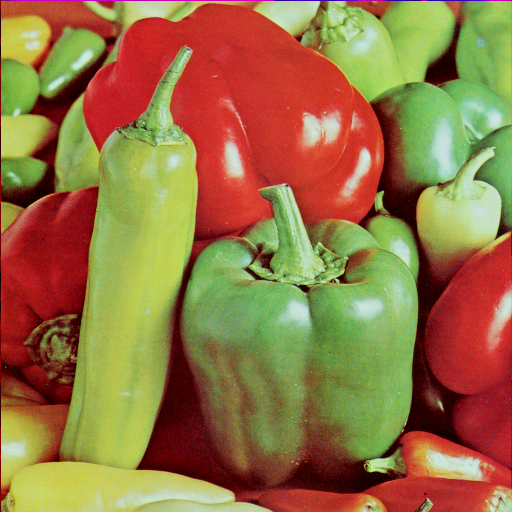}
        \caption{Original image (cropped)}
    \end{subfigure}
    \begin{subfigure}{0.45\linewidth}
        \centering
        \includegraphics[trim={200pt, 50pt, 0pt, 150pt}, clip,width=150pt]{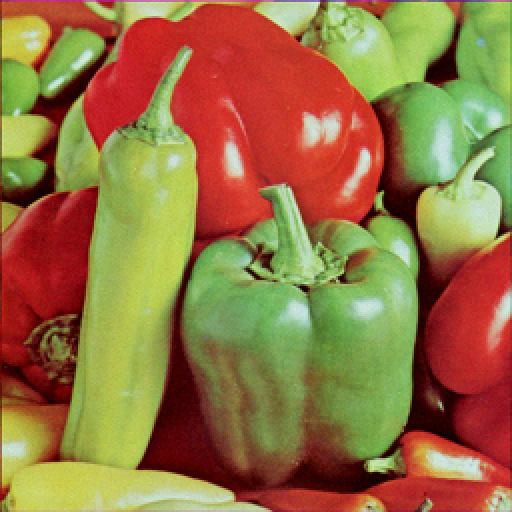}
        \caption{Blurred}
    \end{subfigure}\\
    \begin{subfigure}{0.45\linewidth}
        \centering
        \includegraphics[trim={200pt, 50pt, 0pt, 150pt} ,clip,width=150pt]{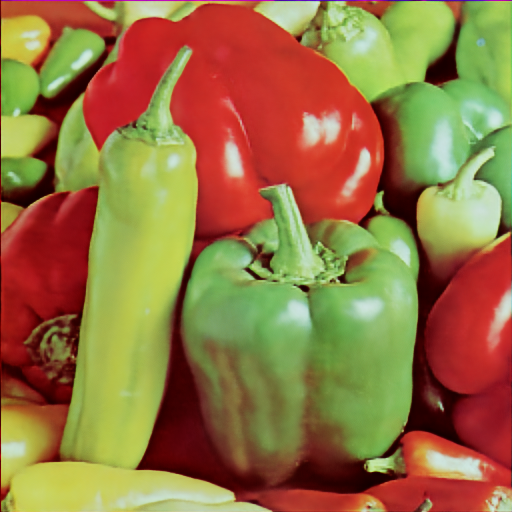}
        \caption{DIP}
    \end{subfigure}
    \begin{subfigure}{0.45\linewidth}
        \centering
        \includegraphics[trim={200pt, 50pt, 0pt, 150pt} ,clip,width=150pt]{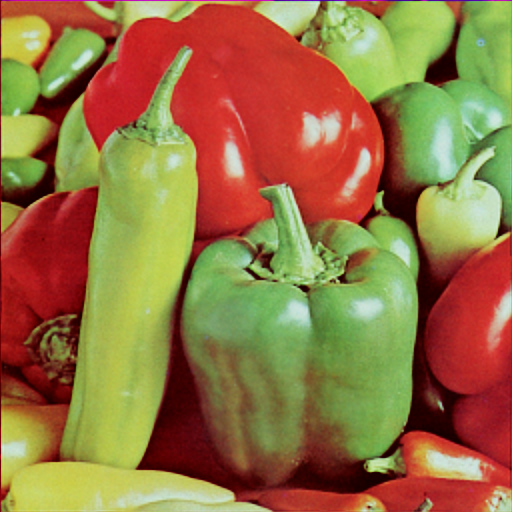}
        \caption{P-GSURE}
    \end{subfigure}\\
    \begin{subfigure}{0.33\linewidth}
        \centering
        \includegraphics[trim={200pt, 50pt, 0pt, 150pt} ,clip,width=150pt]{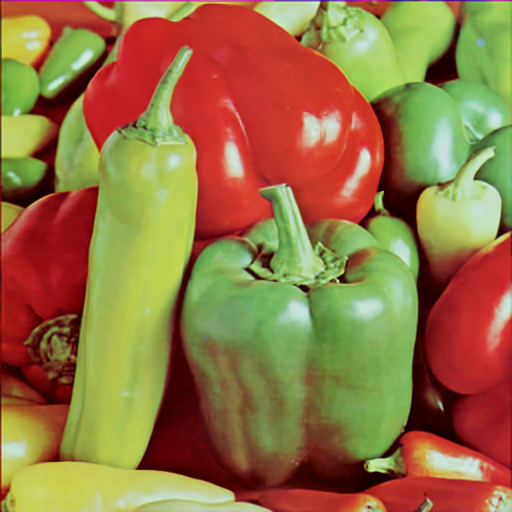}
        \caption{P\&P ADMM}
    \end{subfigure}
    \begin{subfigure}{0.33\linewidth}
        \centering
        \includegraphics[trim={200pt, 50pt, 0pt, 150pt} ,clip,width=150pt]{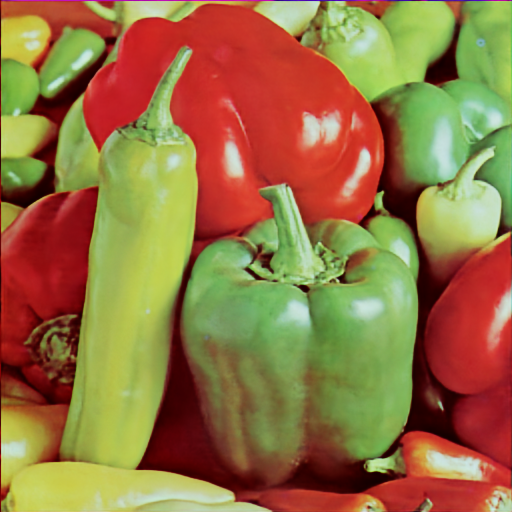}
        \caption{DIP-P\&P}
    \end{subfigure}
    \begin{subfigure}{0.33\linewidth}
        \centering
        \includegraphics[trim={200pt, 50pt, 0pt, 150pt} ,clip,width=150pt]{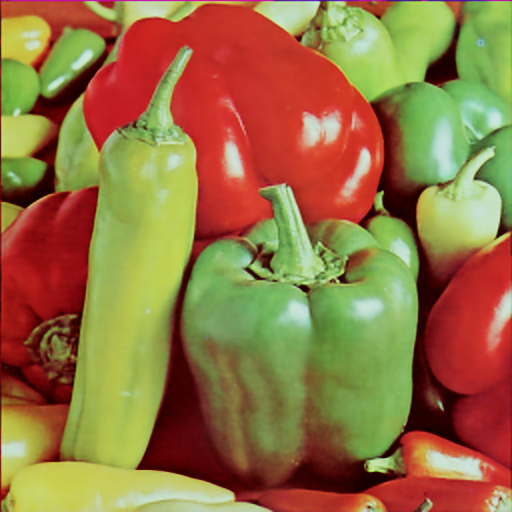}
        \caption{P-GSURE P\&P}
    \end{subfigure}
    \caption{SR of the pepper image from Set14, down-sampled using the model from scenario 3. (a) The original image cropped (b) The observed LR noisy image (c) Reconstruction using DIP (d) Reconstruction using P-GSURE (proposed method) (e) Reconstruction using P\&P-ADMM method (using BM3D prior) (f) Reconstruction using DIP based P\&P-ADMM (g) Reconstruction using P-GSURE based P\&P-ADMM (proposed method).}
    \label{fig:comparison_SR_scenario3}
\end{figure}
